# Supplementary material for: Misbinding Attacks on Secure Device Pairing and Bootstrapping
Source: arXiv:1902.07550 source file (2019-05-31)
Supplement: Supplementary file 1 [file appendix.tex]

% !TeX root = ./main.tex

\section{Bluetooth Model}
\label{sec:bt_model}

\definecolor{comments}{RGB}{2, 112, 10}

\lstset{
    morecomment  = [s][\color{comments}]{(*}{*)},
    keywordstyle = \bfseries\color{blue},
    keywordstyle = [2]\bfseries\color{Magenta},
    keywordstyle = [3]\bfseries\color{comments},
    morekeywords = {among, channel, choice, clauses, const, def, diff, do, elimtrue, else, equation, equivalence, event, expand, fail, forall, foreach, free, fun, get, if, implementation, in, inj-event, insert, let, letfun, new, noninterf, not, nounif, or, otherwise, out, param, phase, pred, proba, process, proof, publicvars, putbegin, query, reduc, secret, set, suchthat, sync, table, then, type, weaksecret, yield},
    basicstyle   = \ttfamily\tiny,
    mathescape   = true,
    frame        = single,
    breaklines   = true,
    numbers      = left,
}

\lstinputlisting{bluetooth.pv}
